# Supplementary material for: Designing Pairwise Interactions that Stabilize Open Crystals: Truncated Square and Truncated Hexagonal Lattices
Source: arXiv:1703.08615 source file (2017-03-24)
Supplement: Supplementary file 1 [file truncs_supplement.pdf]

# Supplemental Material

## I. TRUNCATED HEXAGONAL SPECIAL COMPETITORS

As discussed in the Methods section of the main paper, we illustrate special truncated hexagonal competitors that emerged during the optimization process in figures S1 and S2.

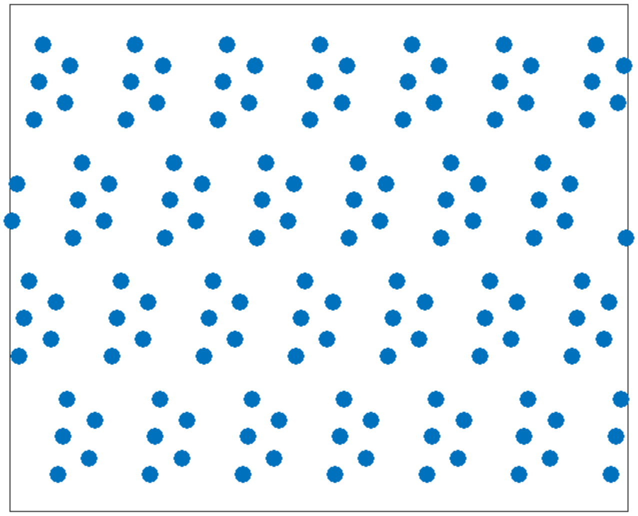

FIG. S1. Special truncated hexagonal competitor consisting of a 5 particle 'cluster' in an oblique lattice

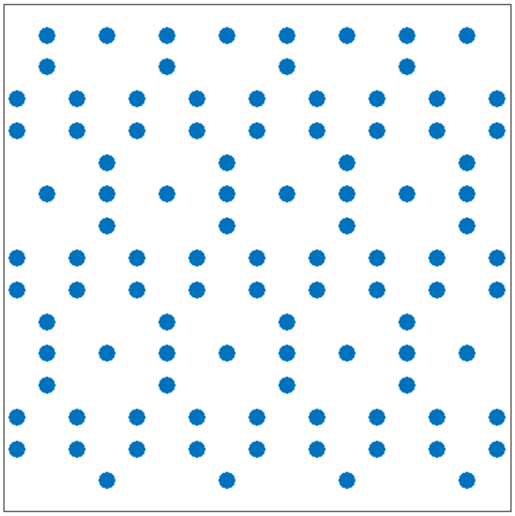

FIG. S2. Special truncated hexagonal competitor consisting of an open decagonal motif with a particle located in the center

## II. PAIR POTENTIAL PARAMETERS OPTIMIZED FOR TRUNCATED SQUARE AND TRUNCATED HEXAGONAL LATTICE

We list the potential parameters of $\phi(r)$ (see eq. 1 in main paper) that maximize the stability (as described in the main text) of truncated square and truncated hexagonal crystal structures. These are listed separately as the parameters of the soft repulsive component and cut off radius and the coefficients of the quadratic components of $f_{\text{shift}}$ in S1. The second table S2 lists the values of $\lambda_i, k_i, d_i$ in the tanh expression up to the appropriate $N_i$ term.

TABLE S1. Parameters $A, n, r_{\text{cut}}$ and $P, Q, R$ for the convex repulsive pair potential $\phi(r)$ found to favor truncated square (TS) or truncated hexagonal (TH) respectively.

| | $A$ | $n$ | $r_{\text{cut}}$ | $P$ | $Q$ | $R$ |
|---|---|---|---|---|---|---|
| TS | $3.44873\times10^{-6}$ | 33.447496 | 3.085443 | -0.218537 | 1.625857 | -3.108286 |
| TH | $2.94536\times10^{-7}$ | 28.078127 | 4.0 | -0.00009071 | 0.00076271 | -0.00160711 |

TABLE S2. Parameters $\lambda_i, k_i, d_i$ for the convex repulsive pair potential $\phi(r)$ found to favor truncated square (TS - $N_i = 2$) or truncated hexagonal (TH - $N_i = 3$) respectively.

| | $\lambda_1$ | $k_1$ | $d_1$ | $\lambda_2$ | $k_2$ | $d_2$ | $\lambda_3$ | $k_3$ | $d_3$ |
|---|---|---|---|---|---|---|---|---|---|
| TS | 2.5 | 0.831795 | 1.081669 | 0.015697 | 6.357929 | 2.584218 | - | - | - |
| TH | 0.314171 | 2.447687 | 1.686265 | 0.149364 | 30.0 | 1.259423 | 0.047484 | 30.0 | 2.472233 |

## III. TRUNCATED HEXAGONAL MONTE CARLO QUENCH RUN

Shown in figure S3 are the Monte Carlo runs of 24 identical seeded crystal systems over approximately 4.6 million Monte Carlo steps as discussed in the methods section of the main paper. Configuration energy in units of $\epsilon$.

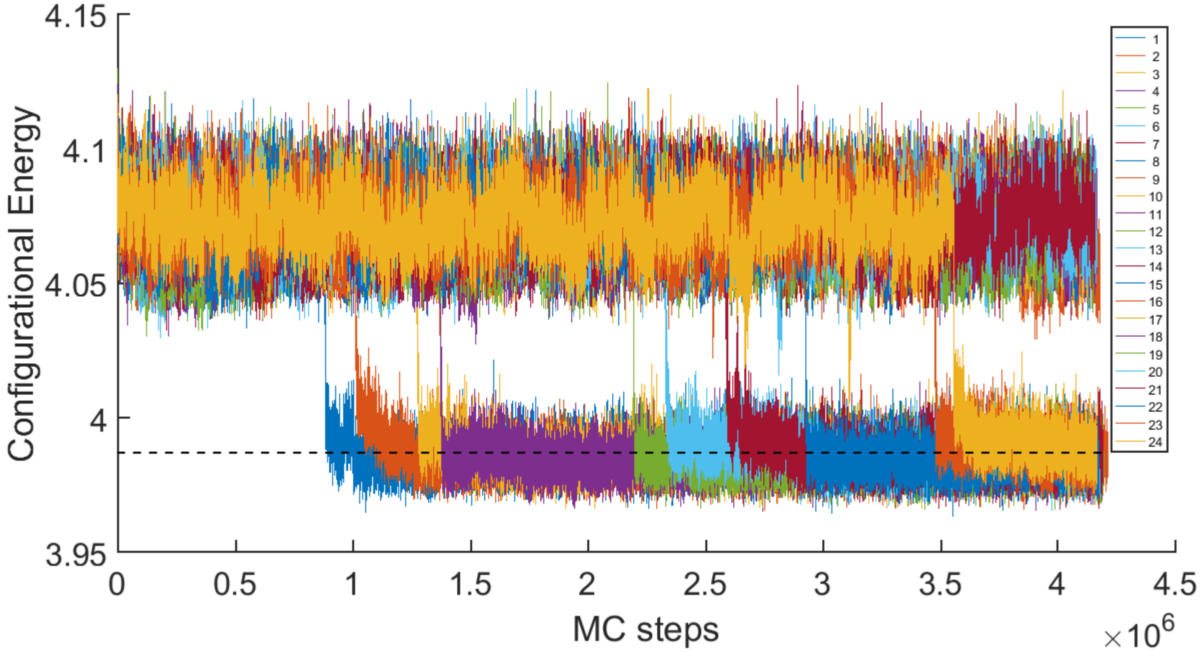


FIG. S3. Monte Carlo quench runs of 24 identical systems using a small frozen crystal seed at $T = 0.06$. Crystallized runs shown sequentially for clarity (15-24). Black dashed line indicates average configuration energy for a perfect crystal at the same temperature.
